# Supplementary material for: Finding Patterns in Ambiguity: Interpretable Stress Testing in the Decision~Boundary
Source: arXiv:2408.06302 source file (2024-08-12)
Supplement: Supplementary file 1 [file X_suppl.tex]

\clearpage
\setcounter{page}{1}
\maketitlesupplementary

\section{Computational Resources}

All experiments were conducted using a machine equipped with a Testa T4 GPU, ensuring sufficient computational power for training and inference phases.

\section{Results}

\todo{If possible to send the suplementary material, write here about the interpretation of this figures and results.}

\begin{table*}[t]
  \centering
  \begin{tabular}{@{}llrrr@{}}
    \toprule
    \multicolumn{2}{c}{\textbf{Dataset}} &  \multicolumn{3}{c}{\textbf{CNN}} \\
    \cmidrule(l){1-2} \cmidrule(l){3-5}
     name  & subset &  nf & accuracy & loss \\
    \midrule
     MNIST & \textit{5 vs 3} & 1 & 92.53\% & 0.23 \\
           &  & 2 & \textbf{92.11\%} & 0.29 \\
           &  & 4 & 96.06\% & 0.10 \\
           & \textit{7 vs 1} & 1 & 97.50\% & 0.09 \\
           &       & 2 & 97.41\% & 0.15 \\
           &       & 4 & 98.84\% & 0.04 \\
           & \textit{8 vs 0} & 1 & 96.31\% & 0.13 \\
           &       & 2 & 95.03\% & 0.16 \\
           &       & 4 & \textbf{98.92\%} & 0.04\\
     Fashion-MNIST & \textit{dress vs top} & 4 & 94.15\% & 0.16\\
           &       & 8 & 94.30\% & 0.16 \\
           &       & 16 & 95.75\% & 0.13 \\
           & \textit{sandal vs sneaker} & 4 &  96.00\% & 0.10 \\
           &       & 8 & 96.70\% & 0.10  \\
           &       & 16 & 97.20\% & 0.07  \\
    \bottomrule
  \end{tabular}
  \caption{Datasets and MUT accuracies. The highlighted values represent the highest and lowest MUT accuracy.}
  \label{tab:accuracies}
\end{table*}

\begin{table*}[t]
  \centering
  \begin{tabular}{@{}llrrrrr@{}}
    \toprule
    \multicolumn{2}{l}{\textbf{Dataset}} & \textbf{CNN} & \multicolumn{3}{c}{\textbf{$ACD < 0.1$}} &  \\
    \cmidrule(l){1-2} \cmidrule(l){3-3} \cmidrule(l){4-6}
    name & subset &  nf & \#test set & \#synthetic & FID synthetic & FID all \\
    \midrule
MNIST         & \textit{5 vs 3}            & 1 & 169          & 2586          & 278.59 & 23.02   \\
              &                            & 2 & \textbf{238} & \textbf{4242} & \textbf{259.83} & 18.80   \\
              &                            & 4 & 60           & 3495          & 325.33 & 98.09   \\
              & \textit{7 vs 1}            & 1 & 37           & 786           & -      & 21.94   \\
              &                            & 2 & 60           & 969           & -      & 17.94   \\
              &                            & 4 & \textbf{11}  & \textbf{364}  & -      & 15.43   \\
              & \textit{8 v 0}             & 1 & 63           & 1605          & -      & 20.84   \\
              &                            & 2 & 75           & 1792          & -      & 20.86   \\
              &                            & 4 & 17           & 673           & -      & \textbf{14.38}   \\
Fashion-MNIST & \textit{dress vs top}     & 4 & 75           & 2421          & 334.59 & \textbf{109.82}  \\
              &                            & 8 & 79           & 2138          & 340.16 & 88.58   \\
              &                            & 16 & 52           & 2024          & \textbf{350.81} & 101.71  \\
              & \textit{sandal vs sneaker} & 4 & 44           & 2904          & 327.78 & 45.88   \\
              &                            & 8 & 32           & 2483          & 338.95 & 48.17   \\
              &                            & 16 & 33           & 2180          & -      & 47.30   \\
    \bottomrule
  \end{tabular}
  \caption{TODO}
  \label{tab:gasten}
\end{table*}

\begin{table*}[t]
  \centering
  \begin{tabular}{@{}lrrrrrrr@{}}
    \toprule
    \textbf{Dataset} & \textbf{CNN} & \multicolumn{3}{c}{\textbf{UMAP}} & \textbf{GMM} & \multicolumn{2}{l}{\textbf{Evaluation}} \\
    \cmidrule(l){1-2} \cmidrule(l){3-5} \cmidrule(l){6-6} \cmidrule(l){7-8}
    subset &  nf & $min\_distance$ & $\#components$ & $\#neighbors$ & $\#clusters$ & SIL ($\uparrow$) & DB ($\downarrow$) \\
    \midrule
\textit{5 vs 3}                & 1  & 0,01 & 60 & 5 & 13 & 0.29          & 1.05          \\
                         & 2  & 0.01 & 60 & 5 & 3  & 0.32          & 1.26          \\
                         & 4  & 0.01 & 60 & 5 & 15 & \textbf{0.26} & \textbf{1.35} \\
\textit{7 vs 1}                & 1  & 0.01 & 60 & 5 & 3  & 0.47          & 0.76          \\
                         & 2  & 0.01 & 5  & 5 & 15 & 0.39          & 0.94          \\
                         & 4  & 0.02 & 20 & 5 & 3  & \textbf{0.52} & \textbf{0.70} \\
\textit{8 vs 0}               & 1  & 0.01 & 5  & 5 & 15 & 0.36          & 0.93          \\
                         & 2  & 0.01 & 11 & 5 & 15 & 0.31          & 1.14          \\
                         & 4  & 0.01 & 5  & 5 & 15 & 0.43          & 0.89          \\
\textit{dress vs top}  & 4  & 0.01 & 60 & 5 & 3  & 0.47          & 0.74          \\
                 & 8  & 0.01 & 51 & 7 & 3  & 0.50          & 0.71          \\
                       & 16 & 0.01 & 5  & 5 & 3  & 0.38          & 1.14          \\
\textit{sandal vs sneaker}  & 4  & 0.01 & 5  & 5 & 15 & 0.27          & 1.19          \\
                       & 8  & 0.04 & 5  & 5 & 3  & 0.33          & 0.96          \\
                        & 16 & 0.01 & 60 & 5 & 15 & 0.28          & 1.12          \\
    \bottomrule
  \end{tabular}
  \caption{Hyperparameters and resulting evaluation metrics for each dataset, where SIL is the silhouette score and DB is the Davies-Bouldin index.}
  \label{tab:hyperparameters}
\end{table*}

\begin{figure}[t]
    \centering
    \includegraphics[width=0.7\linewidth]{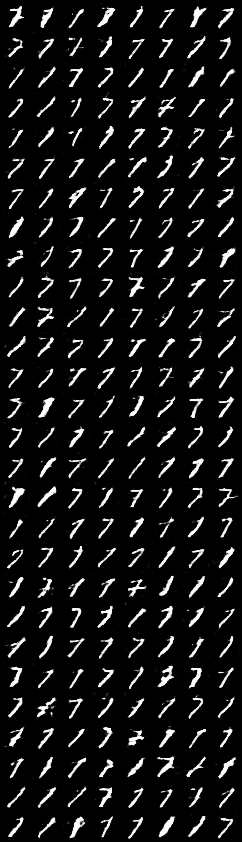}
    \caption{Cluster number 3 of MNIST subset \textit{7 vs 1}}
    \label{fig:one_cluster}
\end{figure}

% this is the 2D baseline vs prototypes
\begin{figure}
  \centering
  \begin{subfigure}{0.5\linewidth}
    \includegraphics[width=\linewidth]{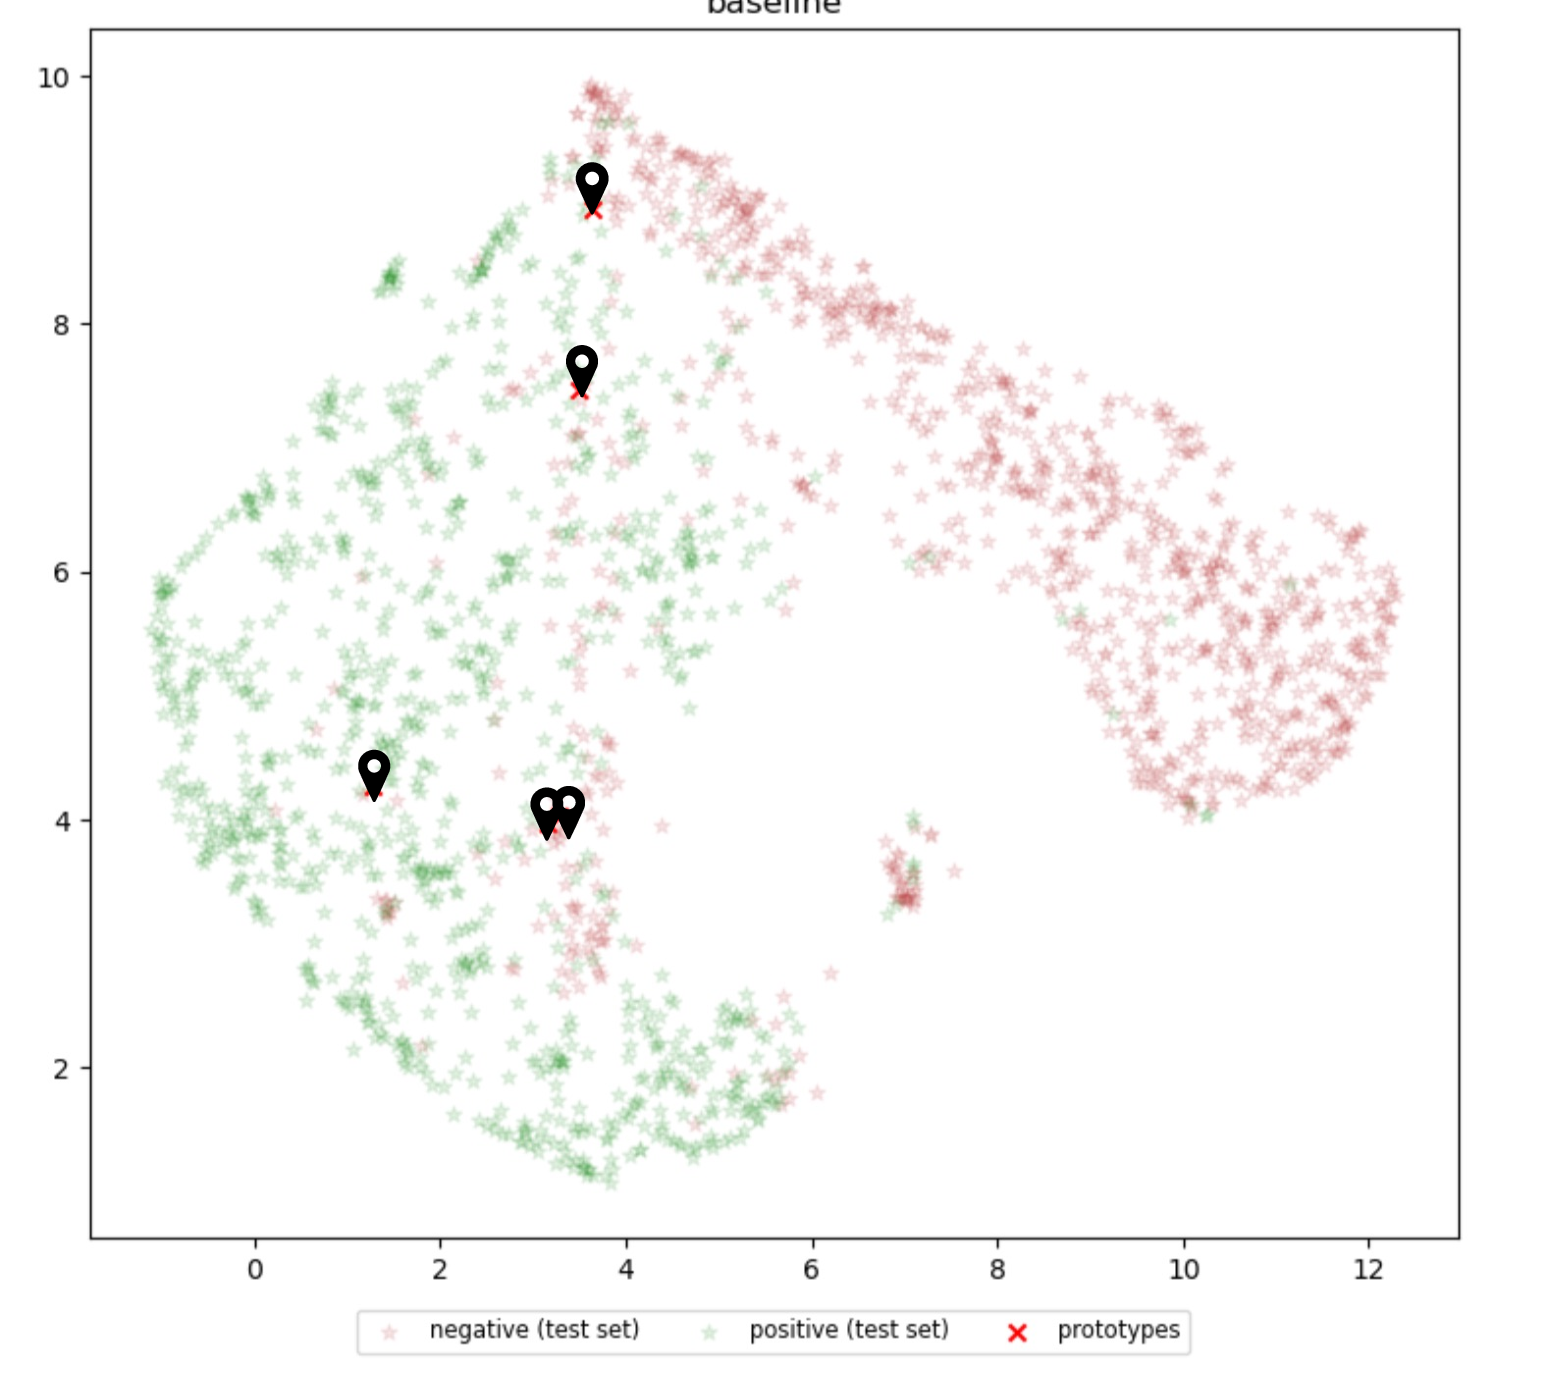}
    \caption{TODO}
    \label{subfig:2dvizbasefashion}
  \end{subfigure}
  \hfill
  \begin{subfigure}{0.48\linewidth}
    \includegraphics[width=\textwidth]{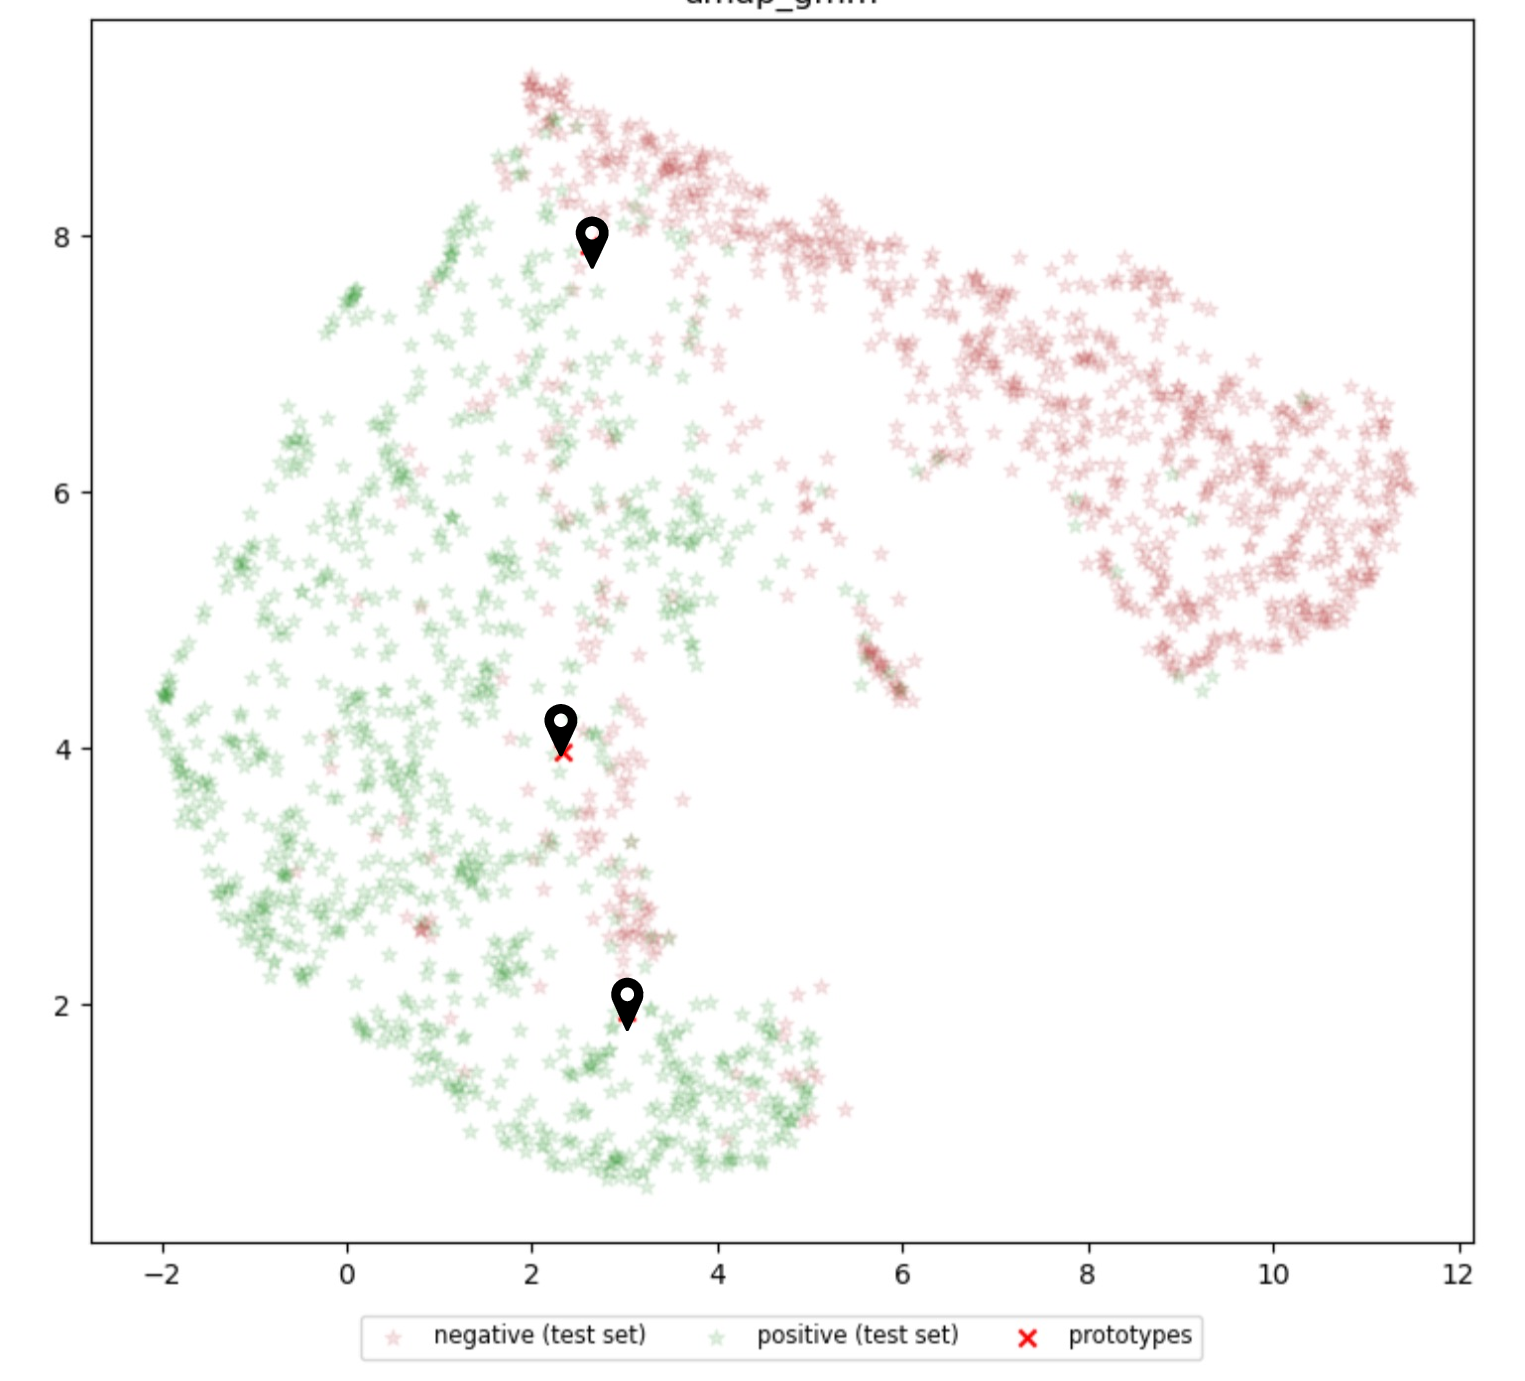}
    \caption{TODO}
    \label{subfig:2dvizprotofashion}
  \end{subfigure}
    \caption{TODO}
  \label{fig:2dviz_fashion}
\end{figure}

% this is the gradientSHAP comparison
\begin{figure}
  \centering
  \begin{subfigure}{0.6\linewidth}
    \includegraphics[width=\linewidth]{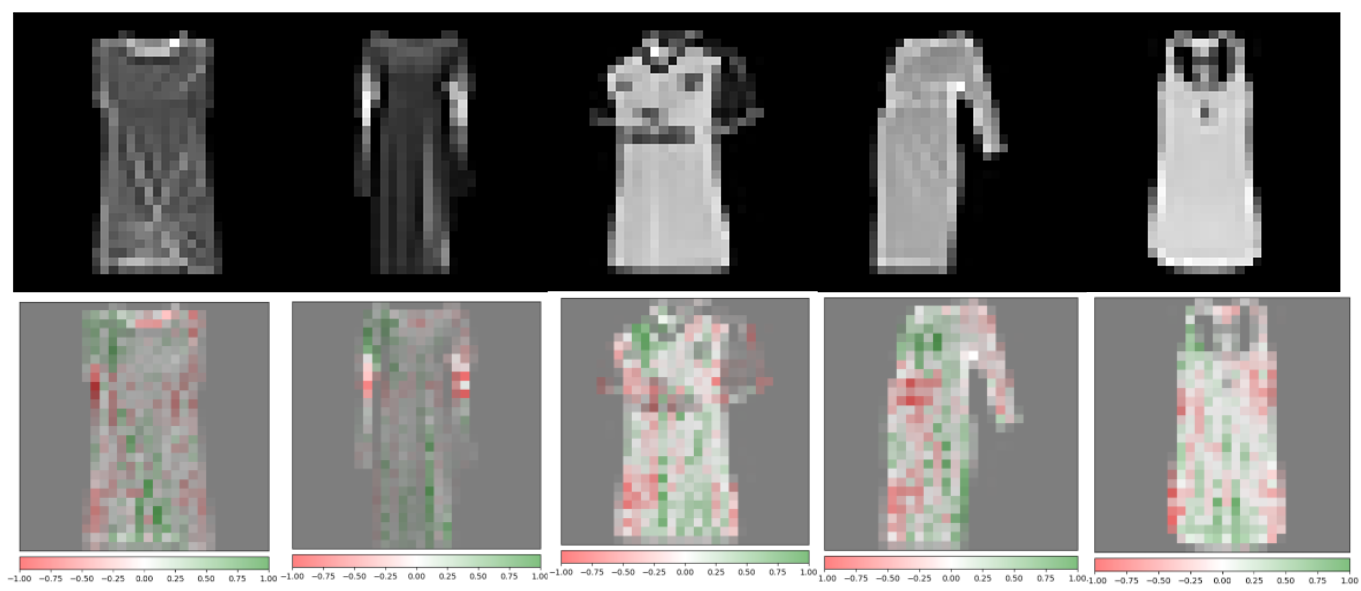}
    \caption{TODO}
    \label{subfig:basefashion}
  \end{subfigure}
  \hfill
  \begin{subfigure}{0.39\linewidth}
    \includegraphics[width=\textwidth]{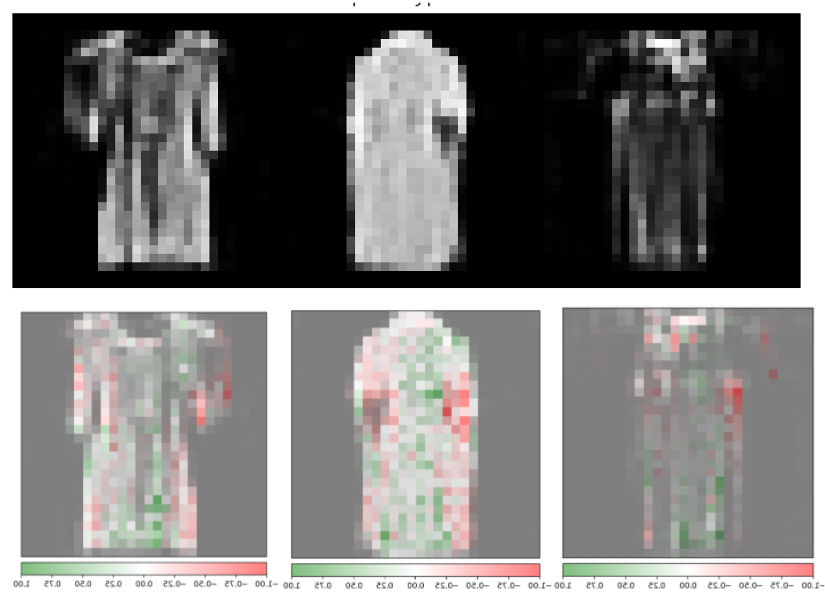}
    \caption{TODO}
    \label{subfig:protofashion}
  \end{subfigure}
    \caption{TODO}
  \label{fig:prototypes_fashion}
\end{figure}
